# Supplementary material for: Continual Learning on Dynamic Graphs via Parameter Isolation
Source: arXiv:2305.13825 source file (2023-07-11)
Supplement: Supplementary file 1 [file PIGNN_Detail.tex]

\subsection{Implementation of PI-GNN}
\label{app:implementation}
\par We introduce the implementation details of PI-GNN. Our implementation is based on \textit{PyTorch Geometric}. All the experiments are conducted on Apple M1 CPU with 8 GB memory. We use GraphSAGE with two layers as the backbone of PI-GNN. For each layer we sample 10 neighbors on Arxiv-S and DBLP-S, and sample 10, 25 neighbors for the first and second layer respectively on Paper100M-S. For Arxiv-S and Paper100M-S, we train our model 400 epochs on the first task and optimize 10 epochs in the knowledge rectification stage and 100 epochs in the parameter isolation stage on later tasks. For DBLP-S we train 600, 40, 100 epochs respectively.
\par The implementation can be described as three parts:
\begin{itemize}
    \item \textbf{Initial training (only for the first task)}: we initialize a GraphSAGE model with 12 hidden units each layer. We train the model on the first snapshot with cross-entropy loss. Learning rate is set as 0.001. We use Adam with weight decay as 0 as the optimizer.
    
    \item \textbf{Knowledge rectification stage (for all tasks except the first one)}: we fine tune the model with the optimization problem \ref{equ:rectify} as 
\begin{equation}
\begin{aligned}
\theta^{t-1}_{stable} = \arg \min_{\theta^{t-1}} \; & L(f_{\theta^{t-1}}(G_{memory}^{t-1})) \\
 - & \beta L(f_{\theta^{t-1}}(G_{unstable}^{t-1})),
\end{aligned}
\end{equation}
    where learning rate is set as 0.001 and we use Adam with weight decay as 0 as the optimizer. Other settings can be found in the \textit{experimental setting} part in our paper.
    
    \item \textbf{Parameter isolation stage (for all tasks except the first one)}: we freeze the parameters got from the knowledge rectification stage and we expand 12 units for each hidden layer. We train the expanded parameters with the optimization problem \ref{parameters isolation optim} as
\begin{equation}
\begin{aligned}
    \min_{\theta_{new}^{t}} \; & L(f_{\theta^{t-1}_{stable}}(\Delta G^{t}) + f_{\theta_{new}^{t}}(\Delta G^{t})) \\& + \lambda \, L(f_{\theta_{new}^{t}}(G_{mems}^{t-1})),
\end{aligned}
\end{equation}
    where learning rate is set as 0.001 and we use Adam with weight decay as 0 as the optimizer. Other settings can be found in the \textit{experimental setting} part in our paper.
\end{itemize}

% \begin{figure*}[h]
% \centering
% \includegraphics[width=0.9\textwidth]{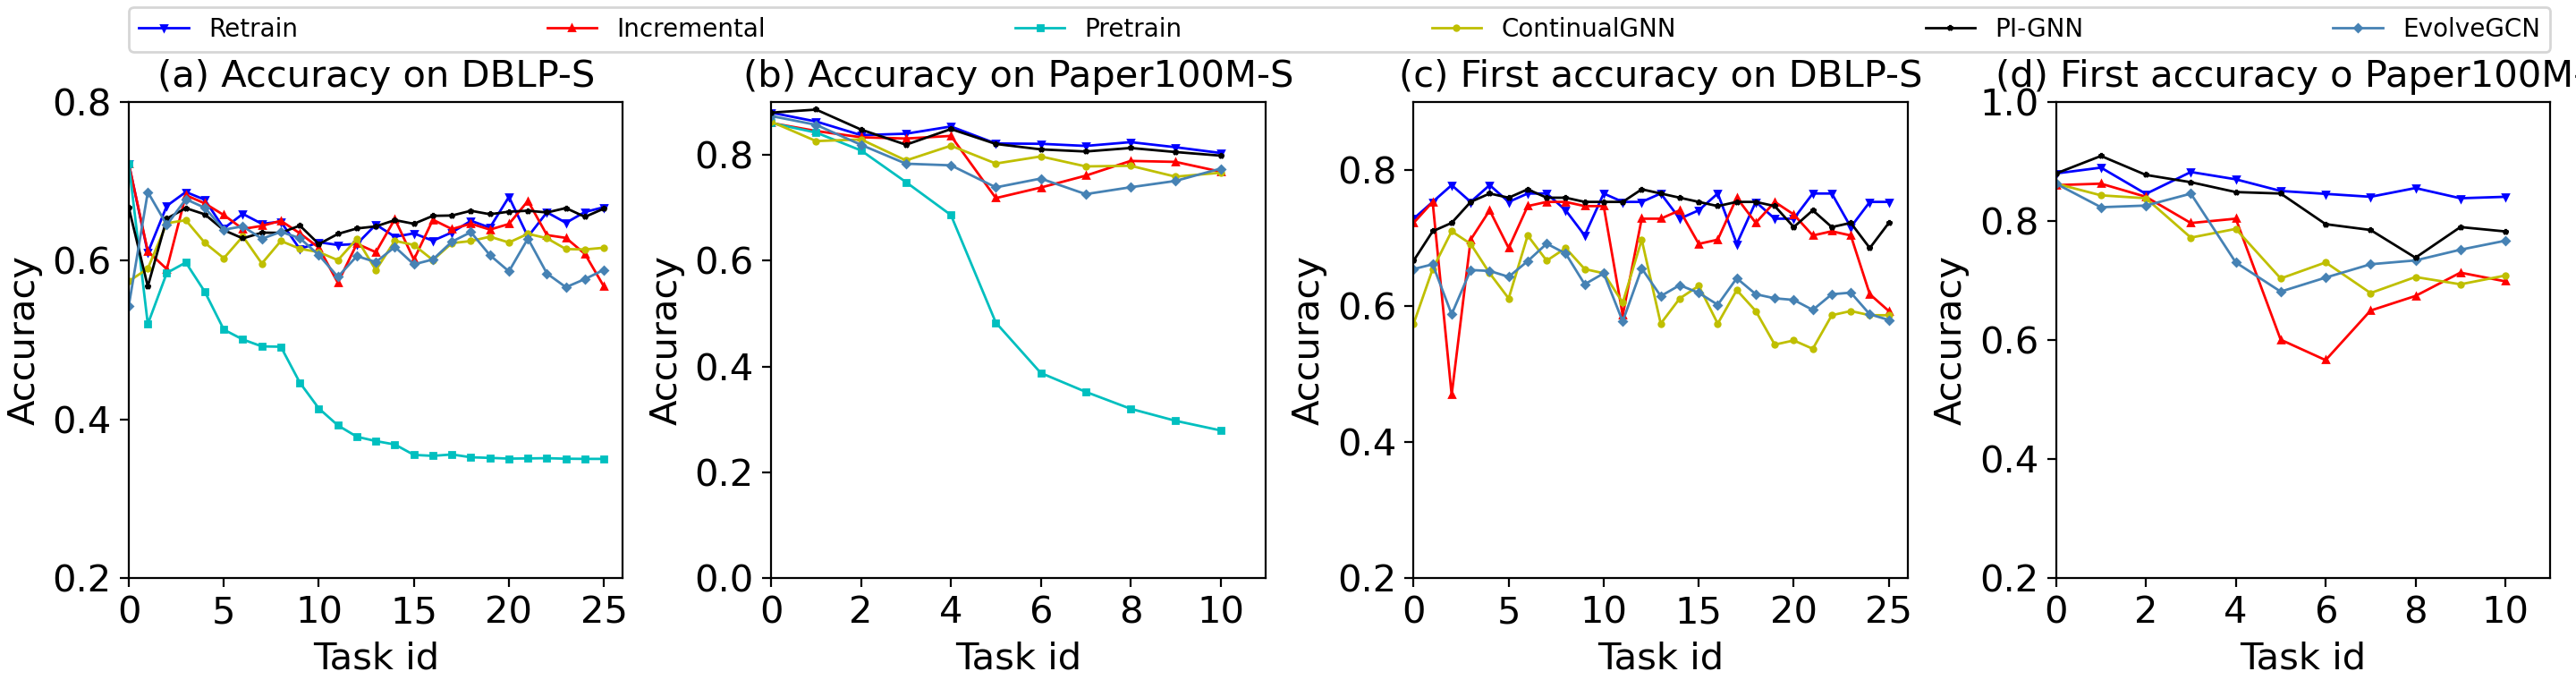}
% \caption{Accuracy on the current task and the first task during learning.}
% \label{figure:appendix_accuracy}
% \end{figure*}
