# Supplementary material for: Continual Learning on Dynamic Graphs via Parameter Isolation
Source: arXiv:2305.13825 source file (2023-07-11)
Supplement: Supplementary file 2 [file baselines_setting.tex]

\subsection{Baselines settings}
\label{app:baseline}
\par We present the setting of our baselines here. The setting can be described as:
\begin{itemize}
    \item \textit{Retrain}: We use the same GNN backbone as PI-GNN and we set the model capacity as the maximal capacity of PI-GNN. For example, if we initialize 12 units, expand 12 units each time and we have 10 tasks, we will set the hidden dimension of \textit{Retrain GNN} as $12*10=120$. The neighbors sample number of each layer is the same as PI-GNN. For each task we use the same training epochs and optimizer as PI-GNN for fairness.
    
    \item \textit{Pretrain}: The setting is the same as \textit{Retrain}
    
    \item \textit{OnlineGNN}: The setting is the same as \textit{Retrain}
    
    \item \textit{EvolveGCN}: We use the official implementation of \textit{EvolveGCN}. we use the version EvolveGCN-O that achieves better performance. We set the model capacity as the maximal capacity of PI-GNN and use the same optimizer as PI-GNN. Other setting is the same as the official reports.
    
    \item \textit{DNE}: We use the official implementation of \textit{DNE}. Because it is a skip-gram based method, thus all the settings are the same as the official reports.
    
    \item \textit{DyGNN}: We use the official implementation of \textit{DyGNN}. Because it has temporal signals. We set the time signal as the timestamps and we use even time interval within a timestamp.  We set the model capacity as the maximal capacity of PI-GNN and use the same optimizer as PI-GNN. Other settings is the same as its official reports.
    
    \item \textit{ContinualGNN}: We use the official implementation of \textit{ContinualGNN}. We set the model capacity as the maximal capacity of PI-GNN and use the same optimizer as PI-GNN. Other settings are the same as its official reports.
    
    \item \textit{DiCGRL}: We use the official implementation of \textit{DiCGRL}. We set the model capacity as the maximal capacity of PI-GNN and use the same optimizer as PI-GNN. Other settings are the same as its official reports.
    
    \item \textit{TWP}: We use the official implementation of \textit{TWP}. We set the model capacity as the maximal capacity of PI-GNN and use the same optimizer as PI-GNN. Other settings are the same as its official reports.
    
\end{itemize}
