# Supplementary material for: Continual Learning on Dynamic Graphs via Parameter Isolation
Source: arXiv:2305.13825 source file (2023-07-11)
Supplement: Supplementary file 3 [file other_model_study.tex]

\subsection{Other Model Analysis Results}
\label{app:other_model_study}

\begin{table}[h]
\centering
\small
\begin{tabular}{c|c|c}
\toprule
\# Rectification Epochs & PM       & FM              \\
\midrule
0            & 72.01$\pm$0.35\%    & \textbf{1.31$\pm$0.43\%}  \\
10           & \textbf{77.02$\pm$0.53\%}    & -1.22$\pm$0.03\% \\
20           & 77.62$\pm$0.32\%    & -1.97$\pm$0.12\% \\
40           & 77.42$\pm$0.64\%    & -0.77$\pm$0.02\% \\
\bottomrule
\end{tabular}
\caption{PM and FM for different \# rectification epochs}
\label{table:appendix_rectification}
\end{table}

\begin{table}[h]
\centering
\small
\begin{tabular}{c|c|c}
\toprule
Methods  & PM    & FM    \\\midrule
No Iso    & 71.96\% & -6.78\% \\
No Exp\&Iso & 68.21\% & -9.25\% \\
PI-GNN   & 77.02\% & -1.22\%  \\
\bottomrule
\end{tabular}
% \caption{PM and FM with/without expansion \& isolation. We do not consider No Expansion because only Isolation makes difficult for model to learn.}
\caption{PM and FM with/without expansion \& isolation.}
\label{table:appendix_isolation}
\end{table}

\begin{table}[h]
\centering
\small
\begin{tabular}{c|c|c|c}
\toprule
Size & PM    & FM    & Average Time(/ms) \\
\midrule
% 32      & 74.52\% & -3.74\% & 20.4             \\
64      & 75.67\% & -2.49\% & 22.2              \\
128     & 77.02\% & -1.22\%  & 24.2              \\
192     & 77.79\% & -0.82\%  & 27.4              \\
256     & 78.31\% & -0.37\%  & 31.2             \\
\midrule
\end{tabular}
\caption{Influence of $G_{memory}$ size.}
\label{table:appendix_sample_num}
\end{table}

\begin{table}[h]
\centering
\small
\begin{tabular}{c|c|c|c}
\toprule
Expansion units number   & PM        & FM        & Average Time(/ms) \\
\midrule
8               & 73.28\%   & -5.70\%   & 22.0              \\
12              & 77.02\%   & -1.22\%   & 24.1              \\
16              & 77.52\%   & -1.68\%   & 26.9              \\
20              & 77.75\%   & -0.80\%   & 30.2              \\
\midrule
\end{tabular}
\caption{Influence of expansion units number.}
\label{table:appendix_expansion_num}
\end{table}

\begin{table}[!t]
\begin{minipage}[!t]{0.48\columnwidth}
  
  \centering
  
  \begin{tabular}{c|c|c}
\toprule
$\beta$   & PM        & FM \\
\midrule
0               & 75.96\%   & -0.17\%   \\
0.01            & 77.02\%   & -1.22\%   \\
0.02            & 76.95\%   & -1.61\%   \\
0.04            & 76.99\%   & -0.87\%   \\
\midrule
\end{tabular}
\caption{Influence of $\beta$.}
  \label{table:appendix_beta_influence}
  \end{minipage}
\begin{minipage}[!t]{0.48\columnwidth}

  \centering
  
  \begin{tabular}{c|c|c}
\toprule
$\lambda$   & PM        & FM \\
\midrule
0              & 75.24\%   & 1.46\%    \\
0.1            & 77.02\%   & -1.22\%   \\
0.2            & 77.22\%   & -0.59\%   \\
0.4            & 76.32\%   & -1.25\%   \\
\midrule
\end{tabular}
\caption{Influence of $\lambda$.}
  \label{table:appendix_lambda_influence}
  \end{minipage}
  \vspace{-0.1cm}
\end{table}

% \begin{table}[h]
% \centering
% \begin{tabular}{c|c|c}
% \toprule
% $\beta$   & PM        & FM \\
% \midrule
% 0               & 75.96\%   & -0.17\%   \\
% 0.01            & 77.02\%   & -1.22\%   \\
% 0.02            & 76.95\%   & -1.61\%   \\
% 0.04            & 76.99\%   & -0.87\%   \\
% \midrule
% \end{tabular}
% \caption{Influence of $\beta$.}
% \label{table:appendix_beta_influence}
% \end{table}

% \begin{table}[h]
% \centering
% \begin{tabular}{c|c|c}
% \toprule
% $\lambda$   & PM        & FM \\
% \midrule
% 0              & 75.24\%   & 1.46\%    \\
% 0.1            & 77.02\%   & -1.22\%   \\
% 0.2            & 77.22\%   & -0.59\%   \\
% 0.4            & 76.32\%   & -1.25\%   \\
% \midrule
% \end{tabular}
% \caption{Influence of $\lambda$.}
% \label{table:appendix_lambda_influence}
% \end{table}

\par We supplement the numerical results of the Model Analysis section in our paper. All the settings are the same as in our paper.

\subsubsection{Rectification Epochs}
\par Table \ref{table:appendix_rectification} shows the influence of different rectification epochs. 
% The PM and FM are shown in Table \ref{table:appendix_rectification}. 
Although no rectification may have less forgetting, it has relative low PM.

\subsubsection{Parameter Isolation Study}
\par We study the importance of parameter isolation in Table \ref{table:appendix_isolation}. We observe that both PM and FM will suffer significant drop upon removal of parameter isolation or expansion.

\subsubsection{Sampling Size Study}
\par Table \ref{table:appendix_sample_num} shows the influence of sampling size. We have the same observation in FM: sampling less nodes may hurt the FM while sampling abundant nodes has little benefits but results in expensive overhead.

\subsubsection{Expansion Units Number Study}
\par We study the influence of expansion units number. The results are shown in Table \ref{table:appendix_expansion_num}. Insufficient expansion hurts the FM while abundant expansion has little benefits on PM and FM but results in expensive overhead.

\subsubsection{Balance Factor Study}
\par We show the influence of balance factor $\beta$ in Table \ref{table:appendix_beta_influence} and $\alpha$ in Table \ref{table:appendix_lambda_influence}. We find that improper balance will have some negative influence on the performance.

\subsubsection{Model Distillation Study}
\par In our paper we show the performance of distilled model and here we give the model size before/ after distillation. The results are shown in Table \ref{table:appendix_distillation}.

\begin{table}[h]
\centering
% \scriptsize
\small
\begin{tabular}{c|c|c|c}
\toprule
\multicolumn{1}{l|}{} & Arxiv-S   & DBLP-S   & Paper100M-S \\
\midrule
PI-GNN Size                & 213KB     & 759KB.    & 285KB \\
Distilled PI-GNN Size      & 47KB      & 47KB.     & 47KB \\
\bottomrule
\end{tabular}
\caption{Model size before/after distillation}
\label{table:appendix_distillation}
\end{table}
