# Supplementary material for: Continual Learning on Dynamic Graphs via Parameter Isolation
Source: arXiv:2305.13825 source file (2023-07-11)
Supplement: Supplementary file 4 [file appendix.tex]

\section{Appendix}
\par In this section, we provide the supplementary materials for our paper.
