# Supplementary material for: Continual Learning on Dynamic Graphs via Parameter Isolation
Source: arXiv:2305.13825 source file (2023-07-11)
Supplement: Supplementary file 6 [file deletion.tex]

\subsection{Node/Edge Deletion}
\label{app:deletion}
\par In this subsection, we generalize PI-GNN to the situation where nodes or edges are deleted. We first generalize the concept of unstable subgraphs, stable subgraphs, and changed subgraphs. In the deletion scenario, we have:
\begin{itemize}
    \item \textbf{Unstable subgraphs $G_{unstable}^{t-1}$} are defined as the $k$-hop ego-subgraphs at snapshot $t-1$ whose center nodes will connect to new/deleted nodes or edges at snapshot $t$.
    \item \textbf{Stable subgraphs $G_{stable}^{t-1}$} are defined as the $k$-hop ego-subgraphs whose center nodes are outside the $k$-hop ranges of nodes connecting to new/deleted nodes or edges at snapshot $t$. 
    \item \textbf{Changed subgraphs $\Delta G^{t}$} are evolved from $G_{unstable}^{t-1}$ after new nodes and edges are added or deleted at snapshot $t$.
\end{itemize}
% We give an illustration in Figure \ref{definition:deletion} to these generalized definitions, especially about node/edge deletions. 

\par Based on these generalized definitions, PI-GNN can also deal with node and edge deletions according to the algorithm described in our paper.
\par Another problem is that if graph patterns disappear significantly due to node and edge deletions, an overly expanded large model may face the overfitting problem. This can be solved by model distillation. If there are too many nodes or edges deleted in dynamic graphs compared to the previous snapshot, we can distill the model to get a smaller model at this snapshot to avoid the overfitting problem. 
% \begin{figure}[t]
%     \centering
%     \includegraphics[width=0.45\textwidth]{appendix_figures/appendix_definition.png}
%     \caption{We use $k=1$ as an example also. At snapshot $t$, node $d$ and edge $(b, c)$ are deleted. Thus, the neighborhoods of $a,b,c$ are the unstable subgraphs at snapshot $t-1$ (denoted by red shades). The unstable subgraphs will become the changed subgraphs after nodes and edges are deleted at snapshot $t$ (denoted by blue shades). The green shades denote the stable subgraphs.}
%     \label{definition:deletion}
% \end{figure}
