# Supplementary material for: Continual Learning on Dynamic Graphs via Parameter Isolation
Source: arXiv:2305.13825 source file (2023-07-11)
Supplement: Supplementary file 7 [file experiment_results.tex]

\subsection{Other Experimental Results and Discussions}
\par In this section we show other experimental results, which consist of: quantitative results on other datasets, average training time of other baselines, results of other backbones and the other model study results.

\begin{table*}[!htbp]
\centering
\begin{tabular}{c|c|cc|cc|cc}
\toprule
                          & Dataset      & \multicolumn{2}{c|}{Arxiv-S}           & \multicolumn{2}{c|}{DBLP-S}        & \multicolumn{2}{c}{Paper100M-S}    \\
\cmidrule{2-8}
                          & Metric             & PM                 & FM                & PM                & FM                & PM               & FM               \\
\midrule
Lower bound                & Pretrain           & 45.99\%            & 0\%               & 43.17\%           & 0\%               & 55.13\%          & 0\%        \\
\midrule
Incremental                & OnlineGNN          & 72.69\%            & -8.57\%           & 63.52\%           & -5.04\%           & 77.70\%          & -6.62\%  \\
\midrule
Dynamic                    & EvolveGCN          & 74.08\%.           & -5.55\%           & 61.52\%           & -4.91\%           & 78.14\%          & -3.17\%  \\
\midrule
Continual                  & ContinualGNN       & 75.36\%.           & -2.17\%           & 62.67\%           &  -0.13\%          & 80.59\%          & -2.02\%    \\
\midrule
Upper bound                & Retrain            & 81.86\%.           & -0.12\%           & 64.77\%           & 1.97\%            & 83.42\%          & -0.64\%    \\
\midrule
\multirow{2}{*}{SAGE}     & PI-GNN              & 77.02\%.           & -1.22\%           & 64.75\%           & -0.64\%           & 83.05\%          & -0.93\%    \\
                          & Distilled PI-GNN    & 76.50\%.           & -1.71\%           & 63.49\%           & -1.11\%           & 82.82\%          & -1.49\%    \\
\midrule
\multirow{2}{*}{GCN}      & PI-GNN              & 76.85\%.           & 0.93\%            & 63.62\%           & -0.89\%           & 82.76\%          & -1.35\%    \\
                          & Distilled PI-GNN    & 76.11\%.           & -0.36\%           & 64.09\%           & 0.57\%            & 82.48\%          & -1.92\%    \\
\midrule
\multirow{2}{*}{GAT}      & PI-GNN              & 78.03\%.           & 1.69\%            & 62.78\%           & -1.55\%           & 82.99\%          & -0.75\%    \\
                          & Distilled PI-GNN    & 76.75\%.           & -1.27\%           & 62.81\%           & -1.57\%           & 82.20\%          & -1.11\%    \\
\bottomrule

\end{tabular}
\caption{Performance Mean (PM) and Forgetting Measure (FM) of different methods for node classification.}
\label{table:other_backbone}
\end{table*}

\subsubsection{Quantitative Results}
\par We show the accuracy and the first task accuracy of DBLP-S and Paper100M-S in Figure \ref{figure:appendix_accuracy}, we make the same observations as in our paper: 
\begin{itemize}
    \item During the training process, PI-GNN is the closest one to \textit{Retrain}, which demonstrates the ability of PI-GNN to adapt to new patterns and coincide with our theoretical analysis. \textit{OnlineGNN} fluctuates greatly because it rewrites parameters and thus suffers from the catastrophic forgetting problem. \textit{Pretrain} can not learn any new patterns thus it performs worst. \textit{OnlineGNN} fluctuates greatly because it rewrites parameters and thus suffers from the catastrophic forgetting problem. \textit{Pretrain} can not learn any new patterns thus it performs worst.
    \item \textit{ContinualGNN} gradually forgets the old knowledge after learning many new patterns because of the constant model capacity, which makes it difficult to accommodate the new patterns using existing parameters without forgetting. \textit{EvolveGCN} can learn on the whole snapshot, but it aims at capturing dynamism of the dynamic graph and will forget inevitably.
    \item It worth noting that on DBLP-S, \textit{OnlineGNN} performs better when preserving the first task knowledge. The reason may be: (i) \textit{ContinualGNN} tries to keep the last task knowledge which makes it hard to relearn the forgetting knowledge, while \textit{OnlineGNN} may relearn the first task knowledge relative easily from new data. (ii) \textit{ContinualGNN} replays many nodes without considering the influence of new data, it indiscriminately regularizes on these data that limits its performance. 
\end{itemize}

\subsubsection{Other Backbone Results}
\par We use different GNN models as the backbones of PIGNN. The results can be found in Table \ref{table:other_backbone}. The other baselines are the same as our paper and we only show \textit{ContinualGNN} and \textit{EvolveGCN} which have best performance in continual learning methods and dynamic learning methods respectively. From Table \ref{table:other_backbone}, our PI-GNN can be combined with different GNN backbones properly.

\begin{figure}[h]
\centering
\includegraphics[width=0.45\textwidth]{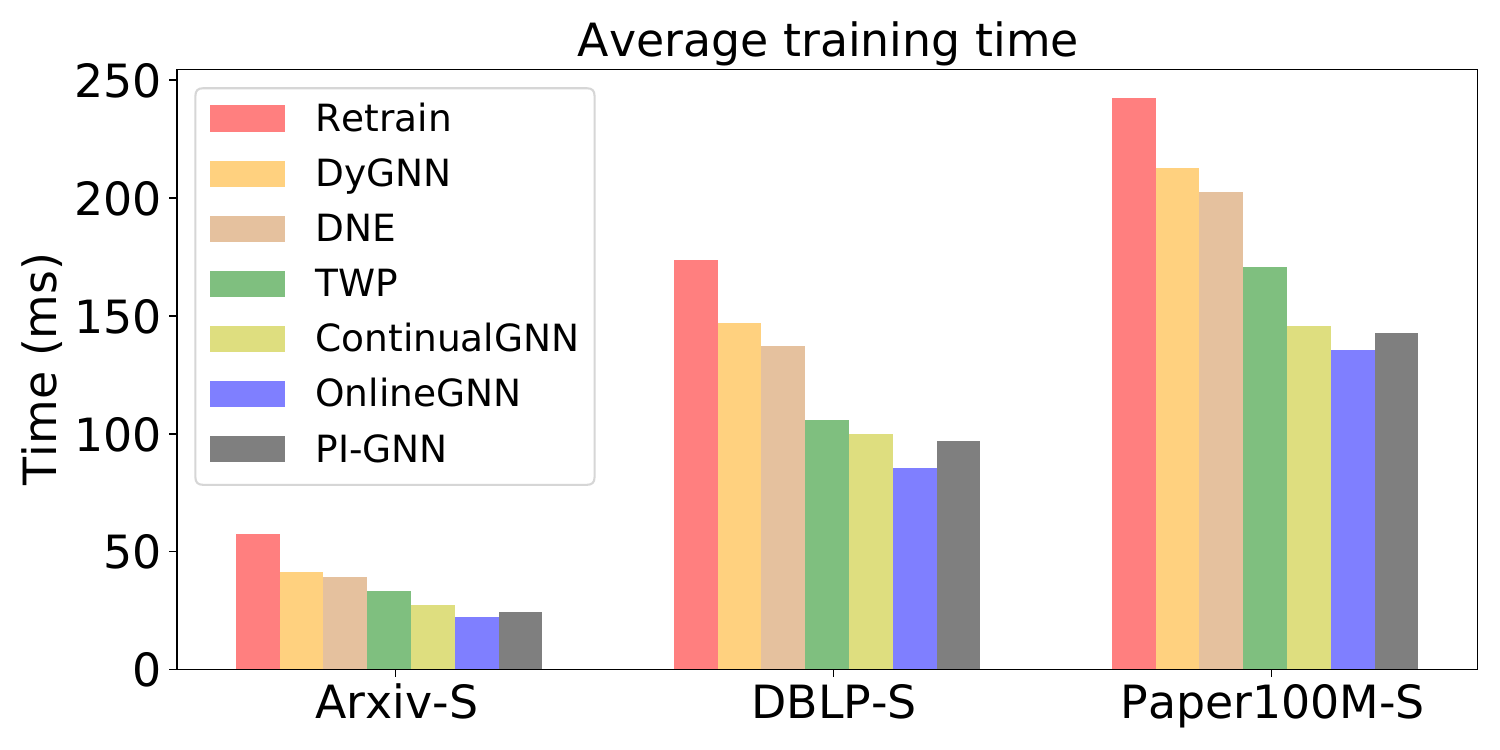}
\caption{Average training time per epoch.}
\label{figure:appendix_efficiency}
\end{figure}

\subsubsection{Efficiency of other baselines}
\par We show the average training time of other baselines in Figure \ref{figure:appendix_efficiency}. We do not show the average training time of \textit{EvolveGCN} because it uses the whole snapshots and RNN to evolve the parameters, which needs more overhead than \textit{Retrain}. \textit{DiCGRL} is not shown here also because it suffers from out of memory problem in Paper100M-S. From the results, we show that PI-GNN is as efficient as \textit{OnlineGNN}. \textit{TWP} has to calculate the topology weights to preserve structure information and thus results in more overheads. It worth noting that \textit{DyGNN} and \textit{DNE} have different settings where they update the nodes embedding after every new edge comes, therefore they have relative large overheads.

\subsubsection{Other Model Study Results}
\par We supplement the numerical results of the Model Study section in our paper. All the settings are the same as in our paper.
\begin{table}[h]
\centering
\small
\begin{tabular}{c|c|c}
\toprule
\# Rectification Epochs & PM       & FM              \\
\midrule
0            & 72.01$\pm$0.35\%    & \textbf{1.31$\pm$0.43\%}  \\
10           & \textbf{77.02$\pm$0.53\%}    & -1.22$\pm$0.03\% \\
20           & 77.62$\pm$0.32\%    & -1.97$\pm$0.12\% \\
40           & 77.42$\pm$0.64\%    & -0.77$\pm$0.02\% \\
\bottomrule
\end{tabular}
\caption{PM and FM for different \# rectification epochs}
\label{table:appendix_rectification}
\end{table}

\textbf{Rectification epochs}
We reports the influence of different rectification epochs. The PM and FM are shown in Table \ref{table:appendix_rectification}. Although no rectification may have less forgetting, it has relative low PM.

\begin{table}[h]
\centering
\small
\begin{tabular}{c|c|c}
\toprule
Methods  & PM    & FM    \\\midrule
No Iso    & 71.96\% & -6.78\% \\
No Exp\&Iso & 68.21\% & -9.25\% \\
PI-GNN   & 77.02\% & -1.22\%  \\
\bottomrule
\end{tabular}
% \caption{PM and FM with/without expansion \& isolation. We do not consider No Expansion because only Isolation makes difficult for model to learn.}
\caption{PM and FM with/without expansion \& isolation.}
\label{table:appendix_isolation}
\end{table}

\textbf{Parameter isolation study}
We study the parameter isolation stage and report the PM and FM in Table \ref{table:appendix_isolation}. We observe that: both PM and FM will suffer significant drop upon removal of parameter isolation or expansion.

\begin{table}[h]
\centering
\small
\begin{tabular}{c|c|c|c}
\toprule
Size & PM    & FM    & Average Time(/ms) \\
\midrule
% 32      & 74.52\% & -3.74\% & 20.4             \\
64      & 75.67\% & -2.49\% & 22.2              \\
128     & 77.02\% & -1.22\%  & 24.2              \\
192     & 77.79\% & -0.82\%  & 27.4              \\
256     & 78.31\% & -0.37\%  & 31.2             \\
\midrule
\end{tabular}
\caption{Influence of $G_{memory}$ size.}
\label{table:appendix_sample_num}
\end{table}

\textbf{Sampling size study}
We study the influence of sampling size. The results are shown in Table \ref{table:appendix_sample_num}. We have the same observation in FM: sampling less nodes may hurt the FM while sampling abundant nodes has little benefits but results in expensive overhead.

\begin{table}
\begin{tabular}{c|c|c|c}
\toprule
Expansion units number   & PM        & FM        & Average Time(/ms) \\
\midrule
8               & 73.28\%   & -5.70\%   & 22.0              \\
12              & 77.02\%   & -1.22\%   & 24.1              \\
16              & 77.52\%   & -1.68\%   & 26.9              \\
20              & 77.75\%   & -0.80\%   & 30.2              \\
\midrule
\end{tabular}
\caption{Influence of expansion units number.}
\label{table:appendix_expansion_num}
\end{table}

\begin{table}
\centering
\begin{tabular}{c|c|c}
\toprule
$\beta$   & PM        & FM \\
\midrule
0               & 75.96\%   & -0.17\%   \\
0.01            & 77.02\%   & -1.22\%   \\
0.02            & 76.95\%   & -1.61\%   \\
0.04            & 76.99\%   & -0.87\%   \\
\midrule
\end{tabular}
\caption{Influence of $\beta$.}
\label{table:appendix_beta_influence}
\end{table}

\begin{table}
\centering
\begin{tabular}{c|c|c}
\toprule
$\lambda$   & PM        & FM \\
\midrule
0              & 75.24\%   & 1.46\%    \\
0.1            & 77.02\%   & -1.22\%   \\
0.2            & 77.22\%   & -0.59\%   \\
0.4            & 76.92\%   & -1.25\%   \\
\midrule
\end{tabular}
\caption{Influence of $\lambda$.}
\label{table:appendix_lambda_influence}
\end{table}

\begin{table}[h]
\centering
% \scriptsize
\small
\begin{tabular}{c|c|c|c}
\toprule
\multicolumn{1}{l|}{} & Arxiv-S   & DBLP-S   & Paper100M-S \\
\midrule
PI-GNN Size                & 213KB     & 759KB.    & 285KB \\
Distilled PI-GNN Size      & 47KB      & 47KB.     & 47KB \\
\bottomrule
\end{tabular}
\caption{Model size before/after distillation}
\label{table:appendix_distillation}
\end{table}

\textbf{Expansion units number study}
We study the influence of expansion units number. The results are shown in Table \ref{table:appendix_expansion_num}. Insufficient expansion hurts the FM while abundant expansion has little benefits on PM and FM but results in expensive overhead.

\textbf{Model distillation study}
\par In our paper we show the performance of distilled model and here we give the model size before/ after distillation. The results are shown in Table \ref{table:appendix_distillation}.
