# Supplementary material for: Continual Learning on Dynamic Graphs via Parameter Isolation
Source: arXiv:2305.13825 source file (2023-07-11)
Supplement: Supplementary file 11 [file other_baselines_discussion.tex]

% \subsection{Baselines Discussion}
% \label{app:baselines_discussion}

% \begin{table*}[!htbp]
% \centering
% \begin{tabular}{c|c|cc|cc|cc}
% \toprule
%                           & Dataset      & \multicolumn{2}{c|}{Arxiv-S}           & \multicolumn{2}{c|}{DBLP-S}        & \multicolumn{2}{c}{Paper100M-S}    \\
% \cmidrule{2-8}
%                           & Metric             & PM                 & FM                & PM                & FM                & PM               & FM               \\
% \midrule
% Lower bound                & Pretrain           & 45.99\%            & 0\%               & 43.17\%           & 0\%               & 55.13\%          & 0\%        \\
% \midrule
% Incremental                & OnlineGNN          & 72.69\%            & -8.57\%           & 63.52\%           & -5.04\%           & 77.70\%          & -6.62\%  \\
% \midrule
% Dynamic                    & EvolveGCN          & 74.08\%.           & -5.55\%           & 61.52\%           & -4.91\%           & 78.14\%          & -3.17\%  \\
% \midrule
% Continual                  & ContinualGNN       & 75.36\%.           & -2.17\%           & 62.67\%           &  -0.13\%          & 80.59\%          & -2.02\%    \\
% \midrule
% Upper bound                & Retrain            & 81.86\%.           & -0.12\%           & 64.77\%           & 1.97\%            & 83.42\%          & -0.64\%    \\
% \midrule
% \multirow{2}{*}{SAGE}     & PI-GNN              & 77.02\%.           & -1.22\%           & 64.75\%           & -0.64\%           & 83.05\%          & -0.93\%    \\
%                           & Distilled PI-GNN    & 76.50\%.           & -1.71\%           & 63.49\%           & -1.11\%           & 82.82\%          & -1.49\%    \\
% \midrule
% \multirow{2}{*}{GCN}      & PI-GNN              & 76.85\%.           & 0.93\%            & 63.62\%           & -0.89\%           & 82.76\%          & -1.35\%    \\
%                           & Distilled PI-GNN    & 76.11\%.           & -0.36\%           & 64.09\%           & 0.57\%            & 82.48\%          & -1.92\%    \\
% \midrule
% \multirow{2}{*}{GAT}      & PI-GNN              & 78.03\%.           & 1.69\%            & 62.78\%           & -1.55\%           & 82.99\%          & -0.75\%    \\
%                           & Distilled PI-GNN    & 76.75\%.           & -1.27\%           & 62.81\%           & -1.57\%           & 82.20\%          & -1.11\%    \\
% \bottomrule

% \end{tabular}
% \caption{Performance Mean (PM) and Forgetting Measure (FM) of different methods for node classification.}
% \label{table:other_backbone}
% \end{table*}


% \par In this section, we give a discussion of baselines. From Table \ref{table:effectiveness}, we have the following analysis for the baselines:
% \begin{itemize}
%     \item \textit{DNE} is even worse than \textit{Pretrain}, because \textit{DNE} do not make use of the node attributes information. 
%     \item \textit{DyGNN} has degenerated performance mainly because it only updates affected node embeddings directly without any strategy to avoid forgetting.
%     \item \textit{EvolveGCN} makes use of \textbf{the whole snapshots} to evolve model parameters and thus have better performance than other dynamic baselines. However, it has no strategy to prevent from the catastrophic forgetting problem, which can be indicated from its FM compared with continual baselines.
%     \item \textit{ContinualGNN} use nodes replay and parameter regularization to deal with forgetting, which has revaltive good performance.
%     \item \textit{TWP} tries to keep the graph structure and parameters to deal with the forgetting problem. In dynamic graph where the structure changes a lot, it is difficult for \textit{TWP} to find an appropriate balance between preserving old knowledge and learning new patterns because it is possible that the graph structure which \textit{TWP} tries to preserve is affected by new data and thus actually hurts the performance of \textit{TWP}.
%     \item \textit{DiCGRL} disentangles the node embeddings and updates the most relevant channel for new relations. Although it can deal with forgetting to some extend, the ability of learning new patterns is also limited because updating only one channel is hard to cover all the new patterns.
%     \item Continual learning baselines suffer less forgetting than dynamic baselines, because continual learning baselines have some strategies to keep old knowledge.
% \end{itemize}
