# Supplementary material for: Continual Learning on Dynamic Graphs via Parameter Isolation
Source: arXiv:2305.13825 source file (2023-07-11)
Supplement: Supplementary file 13 [file other_dataset_results.tex]

\subsection{First Task/Current Task Results of Other Datasets}
\label{app:other_datasets_results}
\par We show the accuracy and the first task accuracy of DBLP-S and Paper100M-S in Figure \ref{figure:appendix_accuracy}, we make the same observations as in our paper: 
\begin{itemize}
    \item During the training process, PI-GNN is the closest one to \textit{Retrain}, which demonstrates the ability of PI-GNN to adapt to new patterns and coincide with our theoretical analysis. \textit{OnlineGNN} fluctuates greatly because it rewrites parameters and thus suffers from the catastrophic forgetting problem. \textit{Pretrain} can not learn any new patterns thus it performs worst. \textit{OnlineGNN} fluctuates greatly because it rewrites parameters and thus suffers from the catastrophic forgetting problem. \textit{Pretrain} can not learn any new patterns thus it performs worst.
    \item \textit{ContinualGNN} gradually forgets the old knowledge after learning many new patterns because of the constant model capacity, which makes it difficult to accommodate the new patterns using existing parameters without forgetting. \textit{EvolveGCN} can learn on the whole snapshot, but it aims at capturing dynamism of the dynamic graph and will forget inevitably.
    \item It worth noting that on DBLP-S, \textit{OnlineGNN} performs better when preserving the first task knowledge. The reason may be: (i) \textit{ContinualGNN} tries to keep the last task knowledge which makes it hard to relearn the forgetting knowledge, while \textit{OnlineGNN} may relearn the first task knowledge relative easily from new data. (ii) \textit{ContinualGNN} replays many nodes without considering the influence of new data, it indiscriminately regularizes on these data that limits its performance. 
\end{itemize}
